# Supplementary material for: High-Resolution Be Aware! Improving the Self-Supervised Real-World Super-Resolution
Source: arXiv:2411.16175 source file (2024-11-25)
Supplement: Supplementary file 1 [file X_suppl.tex]

\clearpage
\setcounter{page}{1}
\maketitlesupplementary
\noindent The supplementary features the following sections:
    \begin{itemize}
    \item Reproduction of LWay~\cite{chen2024low} in \cref{sec:supp_reproduction}.
    \item Design details in \cref{sec:supp_design}, including the architecture of the LR reconstruction network, loss designs, training, and finetuning details.
        
        \item More visual results in \cref{sec:supp_vc}.
        \item Limitations in \cref{sec:supp_lim}.
    \end{itemize}
    
\section{Reproduction of LWay}
\label{sec:supp_reproduction}
Following their official instructions, we reproduce LWay~\cite{chen2024low} based on the code of DegAE~\cite{liu2023degae}. The architecture of the LR reconstruction network exactly follows the details in their paper. Here we demonstrate other details not defined or different from the original paper.

\noindent\textbf{Reconstruction loss $\mathcal{L}_{rec}$} consists of $\ell_1$
loss and LPIPS loss~\cite{zhang2018unreasonable} between the LR inputs and reconstructed LR images:
\begin{equation}
    \mathcal{L}_{rec}(\hat{X}, X) = 
    \lambda_1\mathcal{L}_1(\hat{X}, X) + \lambda_2\mathcal{L}_{LPIPS}(\hat{X}, X),
    \label{eq:supp_rec}
\end{equation}
where $\lambda_1$ and $\lambda_2$ balance the ratio between two loss terms. In all experiments, we set $\lambda_1=1.0$ and $\lambda_2=0.2$.
As stated in \cite{chen2024low}, the pretraining stage directly uses \cref{eq:supp_rec}, and the finetuning stage applies the loss on high-frequency parts of images: $\mathcal{L}_{rec}(\mathrm{W}\odot\hat{X}, \mathrm{W}\odot\!X)$, where $\mathrm{W}\in[0,1]$ is a weight map highlight the high-frequency component of the input image. The detailed implementation of $\mathrm{W}$ is not provided. We apply Haar-based Discrete Wavelet Transform to the reconstructed image $\hat{X}$ and get four channels LL, HL, LH, and HH, where LL includes only low-frequency information in the vertical and horizontal directions. We use normalized summation of absolute values of HL, LH, and HH as the weight map.\\

\noindent\textbf{Dataset for pretraining} in \cite{chen2024low} is a self-collected real-world paired dataset and is not released. Therefore, we synthesize the paired dataset through the second-order degradation pipeline~\cite{wang2021real}. The input LR images include random combinations of Gaussian blur, Gaussian noise, Poisson noise, and JPEG compression. The performance of the reproduced method can be affected by using a pretraining dataset different from that in the original paper. However, our method uses the same synthetic dataset for pretraining for a fair comparison. 

\section{Design Details}
\label{sec:supp_design}
In this section, we introduce detailed implementations of our method, including the architectures of the LR reconstruction network in~\cref{subsec:supp_arch}, the loss functions in~\cref{subsec:supp_loss}, and other details of pretraining and finetuning processes.

\subsection{Architecture of LR reconstruction network}
\label{subsec:supp_arch}
As shown in the main paper~\cref{fig:overview}, the LR reconstruction network in our method consists of a degradation encoder $E_{deg}$, an image encoder $E_{img}$, and a reconstructor $R$. $E_{deg}$ has the same architecture as the degradation encoder in \cite{chen2024low}. The architecture of $E_{img}$ is in \cref{fig:supp_Eimg}, which includes six residual blocks and outputs a 64-channel feature map. The reconstructor $R$ receives input features of 64 channels and the other implementations follow the implementations in \cite{chen2024low}.
\begin{figure}[h!]
    \centering
    \includegraphics[width=0.65\linewidth]{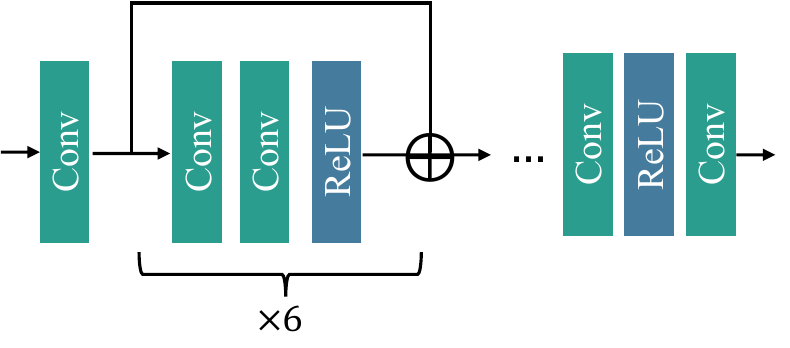}
    \caption{Architecture of image encoder $E_{img}$.}
    \label{fig:supp_Eimg}
\end{figure}

\subsection{Implemention of loss functions} 
\label{subsec:supp_loss}
As shown in the main paper \cref{eq:overview_ft}, our loss design consists of reconstruction loss $\mathcal{L}_{rec}$ and regularizer $\Phi_{far}$. The implementation of $\mathcal{L}_{rec}$ follows \cref{eq:supp_rec} and we use the same design of weight map in \cref{sec:supp_reproduction}.

The regularizer $\Phi_{far}$ calculate distance between features from $E_{img}$ and $E_{clip}$. We use the pretrained CLIP ``RN50" models and take the output of ``layer3" as the output feature of $E_{clip}$. 
% \begin{figure}[h!]
%     \centering
%     \includegraphics[width=0.5\linewidth]{example-image-b}
%     \caption{Architecture of image encoder $E_{clip}$.}
%     \label{fig:supp_Eclip}
% \end{figure}

\input{figures/suppl_visual_cmp_re}
\input{figures/suppl_visual_cmp_swin}
\subsection{Other Details}
\label{subsec:supp_train}
\noindent\textbf{Pretraining details.} The batch size is 16 and weights of $\mathcal{L}_1$, $\mathcal{L}_{LPIPS}$, and $\Phi_{far}$ are 1.0, 0.2, and 0.1 respectively. We train the LR construction network for 500K iterations using two NVIDIA RTX A5000 GPUs.\\

\noindent\textbf{Finetuning details.} The finetuning optimizes the deep part of the parameters of an off-the-shelf SR model. Specifically, for RealESRGAN+~\cite{wang2021real}, we froze the first convolutional layer and the first 20 percent of residual blocks. For SwinIRGAN~\cite{liang2021swinir}, we froze the first convolutional layer and the first 20 percent of Residual Swin Transformer blocks. The weights of $\mathcal{L}_1$ and $\mathcal{L}_{LPIPS}$ are 1.0 and 0.2 for all finetuning cases, and the weight of $\Phi_{far}$ varies between 0.05 and 0.3 depending on the real-world data domains. 

\section{Visual Results}
\label{sec:supp_vc}
More visual comparisons between our methods and other state-of-the-art self-supervised super-resolution methods are shown in~\cref{fig:supp_cmp_re} and ~\cref{fig:supp_cmp_swin}. In general, our method can improve the sharpness of edges and add realistic patterns compared to the other self-supervised methods.

\section{Limitation}
\label{sec:supp_lim}
As shown in \cref{fig:iter}, our method can mitigate overfitting to the reconstruction objective compared to the previous LR reconstruction paradigm. However, the convergence to high-quality high-resolution images needs further proof, and we leave it as future work. Besides, we choose to adjust the primary attribution, the extent, of degradation embeddings, while a finer modification may bring better performance and remains for future exploration.
